# Supplementary material for: Cavitation instabilities in amorphous solids via secondary mechanical perturbations
Source: arXiv:2303.04529 ancillary file (2023-03-08)
Supplement: Supplementary file 1 [file SI.pdf]

# Supplementary information:
# Early onset of cavitation in expanded amorphous solids via secondary deformation

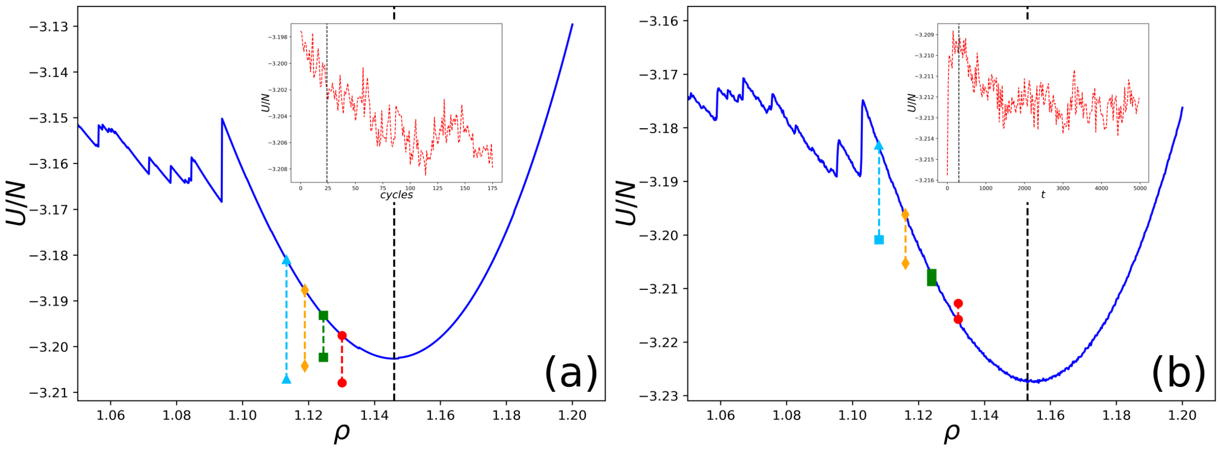


FIG. S1: Evolution of per particle energy ($U/N$) with density ($\rho$) corresponding to the pressure data shown in Fig.2 of the main text, for (a) cyclic shear, (b) active dynamics. In both cases, the dashed vertical line marks the density at which pressure turns negative. In (a), inset shows the stroboscopic variation of energy with cycles after the secondary deformation is imposed on the state (obtained during expansion) at $\rho =$ for (marked with red dotted line in the main figure). In (b), the inset shows the variation of energy with time when activity is imposed on the state (obtained during expansion) at $\rho =$ for (marked with red dotted line in the main figure).

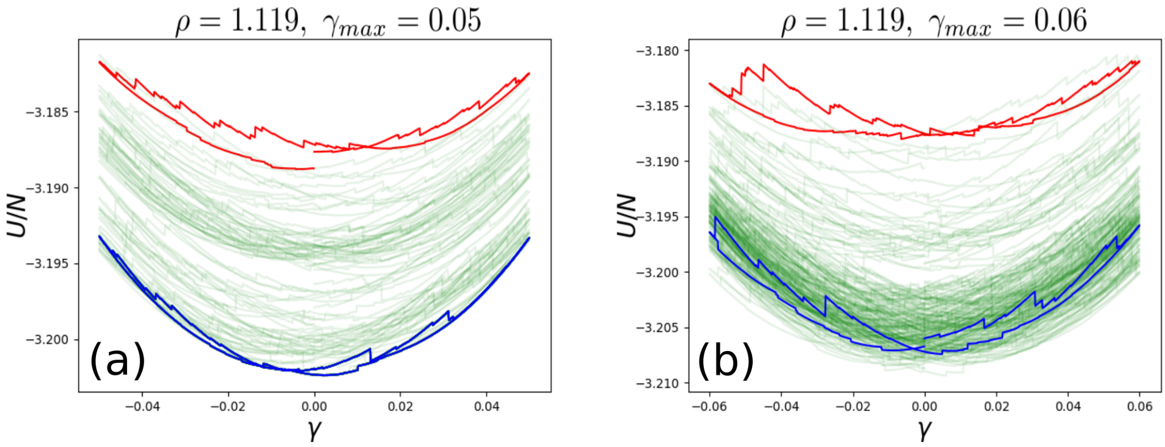


FIG. S2: **Cyclic shear.** Energy within cycles of cyclic shear when cavitation occurs. Red curve shows the first cycle and the blue curve shows the last cycle (a) For an absorbing state with cavity $\gamma_{max} < \gamma_{yield}$ (b) For $\gamma_{max} > \gamma_{yield}$, the system doesn't reach a stuck state and the cavity shape keeps evolving.

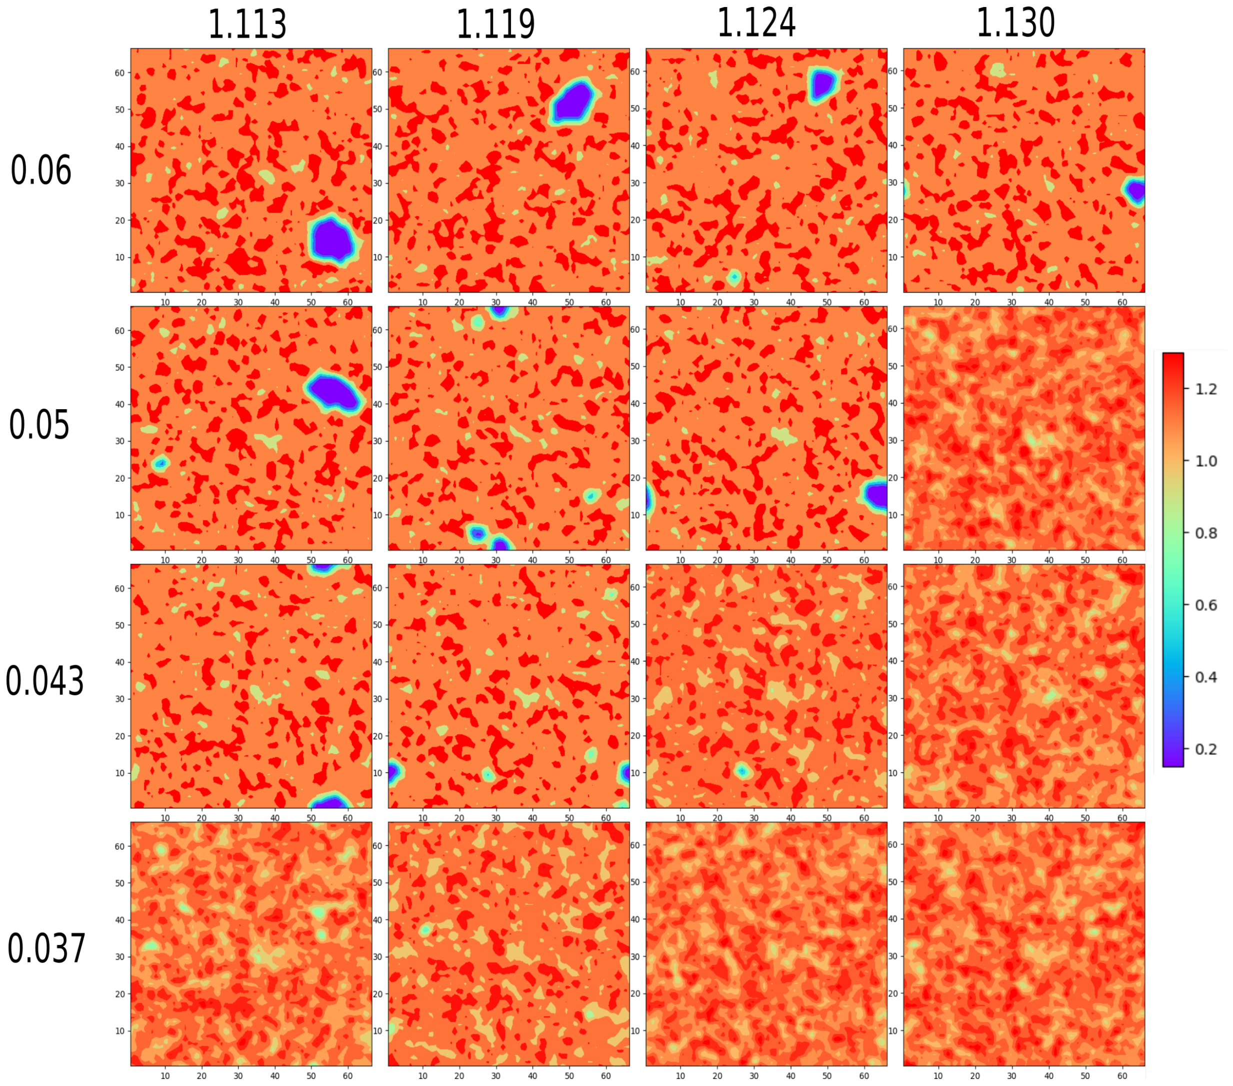


FIG. S3: **Cyclic shear.** Maps of coarse-grained local density, for different densities (x-axis) and amplitudes of cyclic shear (y-axis), as marked. Maps are generated at the end of 200 cycles.

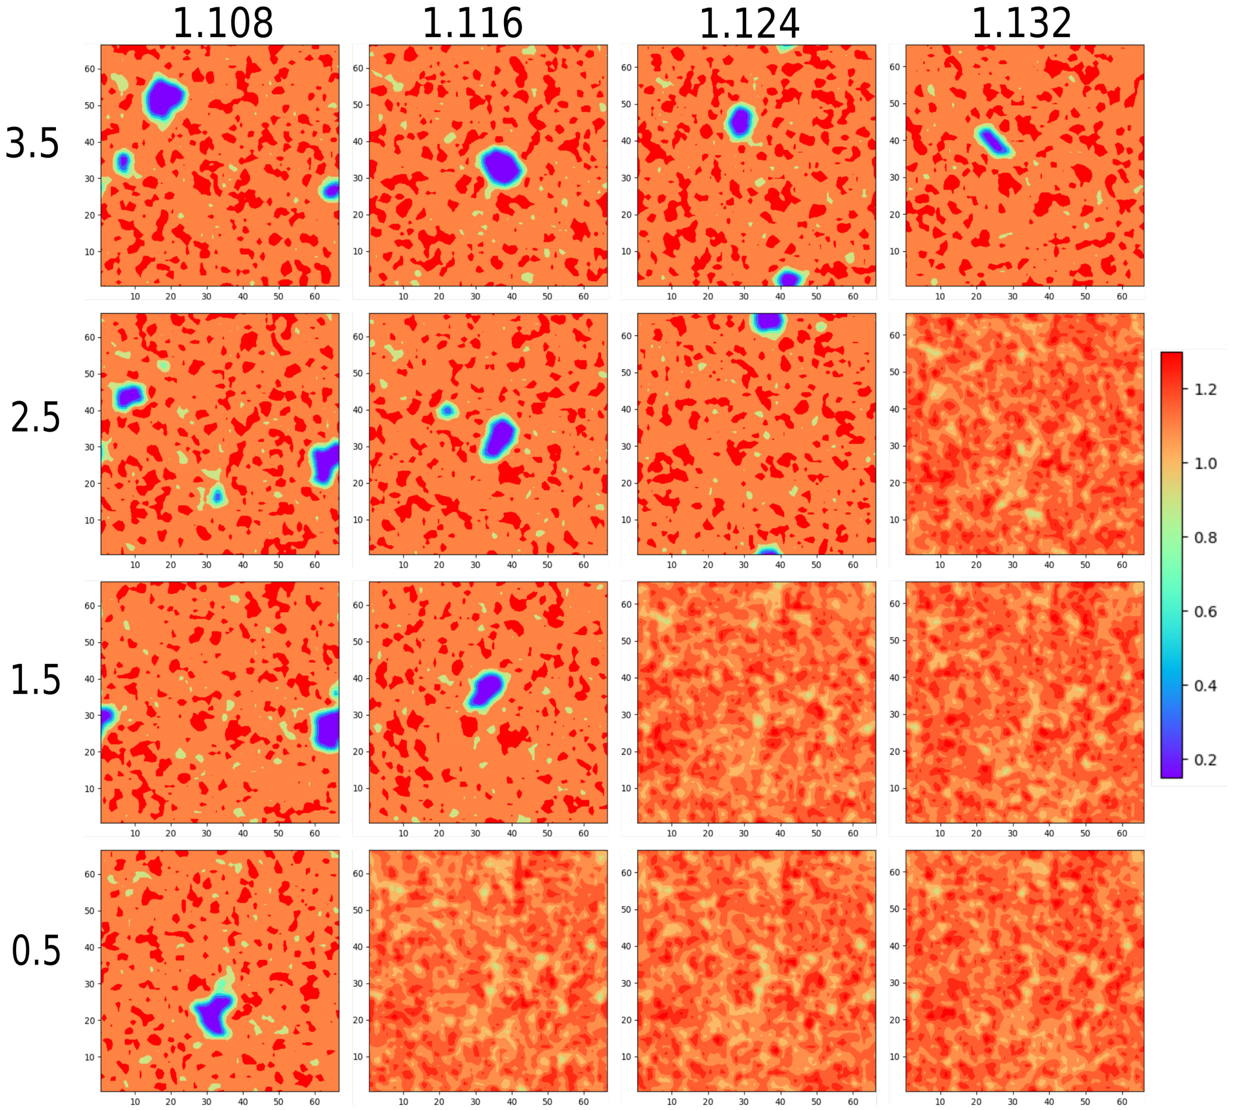


FIG. S4: **Active dynamics.** Maps of coarse-grained local density, as a function of overall density (x-axis) and magnitude of active forcing (y-axis).

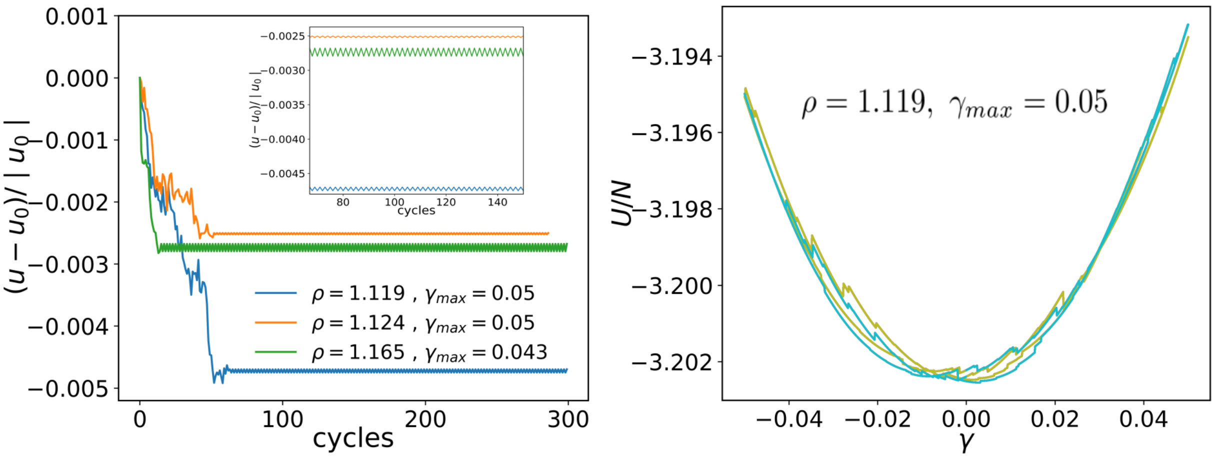


FIG. S5: **Cyclic shear.** Examples of observed limit cycles with period two. (Left): Stroboscopic energy per particle vs cycles, with the inset zooming in to show the bistability. (Right): Energy per particle within the shear cycle for one of the cases shown in the left.

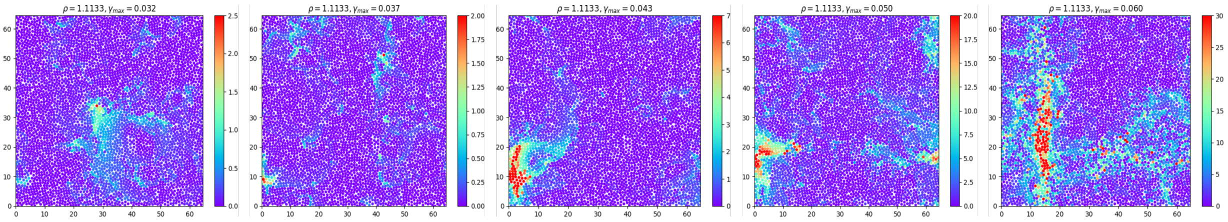


FIG. S6: **Cyclic shear.** Mobility maps at $\rho = 1.1133$, for different shear amplitudes as labelled, starting from same initial state.

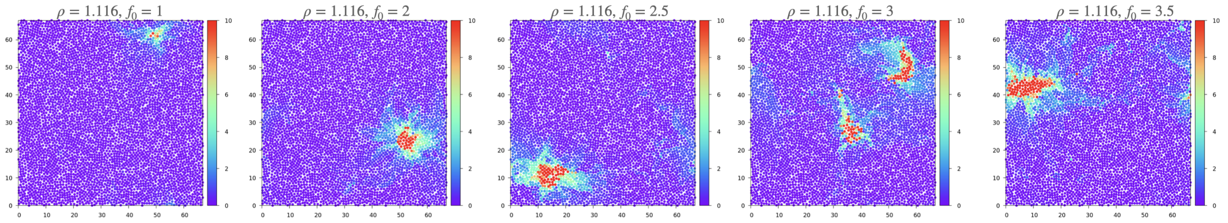


FIG. S7: **Active dynamics.** Mobility maps measured at $\rho = 1.116$ for different magnitudes of forcing $f_0$ as labelled, starting from same initial state.
